# Supplementary material for: Spin-Wave Quantum Computing with Atoms in a Single-Mode Cavity
Source: arXiv:2109.15252 source file (2021-09-30)
Supplement: Supplementary file 1 [file SupplementalMaterial.pdf]

# Supplemental Material: Spin-Wave Quantum Computing with Atoms in a Single-Mode Cavity

Kevin C. Cox,[1,*] Przemyslaw Bienias,[2] David H. Meyer,[1] Paul D. Kunz,[1] Donald P. Fahey,[1] and Alexey V. Gorshkov[2]

[1]*DEVCOM Army Research Laboratory, Adelphi, MD 20783 USA*

[2]*Joint Quantum Institute and Joint Center for Quantum Information and Computer Science, NIST/University of Maryland, College Park, Maryland 20742, USA*

(Dated: September 30, 2021)

### A. Introduction

In this supplemental document, we first, in Sec. B, derive the effective atom-cavity Hamiltonian in Eq. (5) of the main text. Next, in Sec. C, we briefly derive the leading fundamental sources of error in a spin-wave beamsplitter, due to atomic saturation (Sec. C 1), free space emission (Sec. C 2), and cavity emission (Sec. C 3).

### B. Atom-cavity Hamiltonian

In this section, we derive the effective detuned atom-cavity Hamiltonian. The atom-cavity system is goverened by the Tavis-Cummings Hamiltonian

$$\hat{H}_c = \hbar\delta\hat{c}^\dagger\hat{c} + \hbar g(\hat{c}^\dagger\,\hat{J}_- + \hat{c}\,\hat{J}_+), \tag{S1}$$

where $\hat{c}$ is the cavity field operator, and $\hat{J}_- = \sum_{i=0}^{N-1}|g_i\rangle\langle e_i|$ and $\hat{J}_+ = \sum_{i=0}^{N-1}|e_i\rangle\langle g_i|$ are the collective atomic lowering and raising operators. The Hamiltonian is written in the rotating frame of the atomic transition. The Heisenberg equations of motion are

$$\dot{\hat{c}} = -i\delta c - ig\hat{J}_-, \tag{S2}$$

$$\dot{\hat{J}}_- = -igN\hat{c}. \tag{S3}$$

In the limit of large detuning, $|\delta| \gg g\sqrt{N}$, we adiabatically eliminate the cavity to obtain:

$$\hat{c} \approx -\frac{g}{\delta}\hat{J}_-. \tag{S4}$$

Inserting this into Eq. (S3), we obtain

$$\dot{\hat{J}}_- = i\frac{g^2}{\delta}N\hat{J}_-, \tag{S5}$$

which can be generated by an effective Hamiltonian

$$\hat{H}_0^k = -\hbar\frac{g^2}{\delta}\hat{J}_+\hat{J}_-. \tag{S6}$$

If the number of excitations is low, the atomic raising and lowering operators may be approximated as harmonic creation and annihilation operators, giving rise to

$$\hat{H}_0^k = -\hbar\frac{\Omega^2}{4\delta}\hat{b}_0^\dagger\hat{b}_0, \tag{S7}$$

where $\hat{b}_0 \approx \hat{J}_-/\sqrt{N}$ and $\Omega = 2g\sqrt{N}$ is the vacuum Rabi splitting.

### C. Fundamental beamsplitter errors

In this section, we briefly discuss the scale of fundamental errors that arise in the beamsplitter operation $\hat{H}^{BS}$ [see Eq. (6) of the main text],

$$\hat{H}^{BS} = -\hbar\frac{\Omega^2}{4\delta}(\hat{b}_0^{\dagger A} + \hat{b}_0^{\dagger B})(\hat{b}_0^A + \hat{b}_0^B). \tag{S8}$$

Three sources of error are considered: atomic saturation (Sec. C 1), free space emission (Sec. C 2), and cavity emission (Sec. C 3).

#### 1. Atomic Saturation

Atomic saturation induces error in a spin-wave beamsplitter through the introduction of anharmonicity that leads to deviations from a linear beamsplitter. The scaling of this error can be derived from the Holstein-Primakoff transformation [S1], $\hat{J}_+ = \sqrt{N}\hat{b}_0^\dagger\sqrt{1-\frac{\hat{b}_0^\dagger\hat{b}_0}{N}}$, $\hat{J}_- = \sqrt{N}\sqrt{1-\frac{\hat{b}_0^\dagger\hat{b}_0}{N}}\hat{b}_0$. The atom-cavity Hamiltonian of Eq. (S6) can then be written as

$$\hat{H}_0^k \propto \hat{b}_0^\dagger\hat{b}_0 - \frac{\hat{b}_0^\dagger\hat{b}_0^\dagger\hat{b}_0\hat{b}_0}{N}. \tag{S9}$$

If we assume that mode $\hat{b}_0$ is occupied by $m$ excitations, the relative size of the second term (the error) of this Hamiltonian scales as $m/N$. This Hamiltonian leads to the following equation of motion describing $\hat{b}_0$,

$$\dot{\hat{b}}_0 \propto i(\hat{b}_0 - \frac{2}{N}\hat{b}_0^\dagger\hat{b}_0\hat{b}_0). \tag{S10}$$

The second (error) term in Eq. (S10) leads to an erroneous phase accumulation in $\hat{b}$ of magnitude $2(m-1)/N$, that leads to a beamsplitter error (one minus fidelity) of $E_M \sim (m-1)^2/N^2$. For the unitary beamsplitters and phase shifts we consider here, the loss in fidelity due to anharmonicity always scales quadratically since the error is being expanded around a minimum. For Fig. 3 of the main text, we assume the worst case scenario for the

* Corresponding author: kevin.c.cox29.civ@army.mil

anharmonicity error, by assuming that $m$ scales linearly with the mode capacity $M$, $m \propto M$.

In the future, it may be possible to devise a spin-wave quantum computing scheme that can operate outside of the linear regime, and avoid this error. For this work, we choose to treat anharmonicity as an error that negatively affects the figure of merit of the spin-wave processor in Fig. 3 of the main text.

### *2. Free Space Emission*

We now consider errors due to free-space emission while the atom-cavity coupling is turned on for the duration of a beamsplitter operation. Atoms emit into free space with probability $P = \Gamma T$, where the beamsplitter is applied for a time $T \sim \delta/\Omega^2$, leading to an error

$$E_{FS} \sim \frac{\Gamma \delta}{\Omega^2}. \tag{S11}$$

This error scales as the ratio of the loss rate $\Gamma$ and the strength of the Hamiltonian in Eq. (S6). This error decreases for smaller detunings $\delta$.

### *3. Cavity Emission Error*

Next, we calculate the error that results from atoms emitting into the cavity mode during a beamsplitter operation. For a far-detuned cavity, the emission rate $\Gamma_c$ into the cavity mode is

$$\Gamma_c \sim \kappa \frac{\Omega^2}{\delta^2}, \tag{S12}$$

where $\kappa$ is the cavity decay rate and $\frac{\Omega^2}{\delta^2}$ represents the intracavity photon number. The resulting error $E_c$ is of order $\Gamma_c T$ with the beamsplitter being applied for $T \sim \delta/\Omega^2$, leading to

$$E_c \sim \Gamma_c T \sim \frac{\kappa}{\delta}. \tag{S13}$$

This error improves with larger detunings $\delta$, that may be increased up to the cavity free spectral range $\delta_{max} \sim FSR$. Therefore, the smallest fractional error in a beamsplitter or collective phase shift reduces to $E_c \sim 1/f$ for an optical cavity with finesse $f$. However, the optimum detuning is one that sets $E_{FS}$ and $E_c$ equal. This optimum detuning is

$$\delta_{opt} \sim \Omega \sqrt{\frac{\kappa}{\Gamma}} = \sqrt{NC}\kappa. \tag{S14}$$

At the optimum detuning, the errors are

$$E_{FS} \sim E_c \sim 1/\sqrt{NC}. \tag{S15}$$

These errors are summed to evaluate the maximum capacity in Fig. 3 of the main text.

[S1] T. Holstein and H. Primakoff, "Field Dependence of the Intrinsic Domain Magnetization of a Ferromagnet," Physical Review **58**, 1098–1113 (1940).
